# Supplementary material for: Reaching the Limit in Autonomous Racing: Optimal Control versus Reinforcement Learning
Source: arXiv:2310.10943 source file (2023-10-18)
Supplement: Supplementary file 1 [file appendix.tex]

\appendix

\setcounter{figure}{0}

\setcounter{table}{0}

\subsection*{Supplementary Materials for}

\textbf{Reaching the Limit in Autonomous Racing: Optimal Control versus Reinforcement Learning} \\

\noindent Yunlong Song$^{1}$, Angel Romero$^{1}$, Matthias M\"uller$^{2}$, Vladlen Koltun$^{2}$, Davide Scaramuzza$^{1}$ \\

\noindent $^{1}$ University of Zurich, Switzerland\\
\noindent $^{2}$ Intel Labs

\clearpage

\subsection*{Supplementary Methods}

\rebuttal{

\subsection*{Quadrotor Dynamics}
The quadrotor is modeled as a rigid body that is actuated by four motors. 
The quadrotor state is described using a state vector $\mathbf{s} = [\mathbf{p}_W, \mathbf{q}_W, \mathbf{v}_W, \boldsymbol{\omega}_B]$, where $W$ and $B$ indicate the world frame and body frame separately. 
Here, $\mathbf{p}_{W}$ is the position, $\mathbf{q}_{W}$ is a unit quaternion, $\mathbf{v}_{W}$ is the linear velocity, and $\boldsymbol{\omega}_{B}$ is the body rates.
We use the following dynamical model to describe the quadrotor's motion:
\begin{align*}
\mathbf{\dot{p}}_{W} &= \mathbf{v}_{W}   & 
\mathbf{\dot{v}}_{W} &= \mathbf{q}_{W} \odot \mathbf{c} - \mathbf{g} - \mathbf{RDR}^T\mathbf{v}_W \\
\mathbf{\dot{q}}_{W} &= \frac{1}{2} \mathbf{\Lambda} ( \boldsymbol{\omega}_{B}) \cdot \mathbf{q}_{W}   & 
\boldsymbol{\dot{\omega}}_{B} &= \mathbf{J}^{-1} (\boldsymbol{\eta} - \boldsymbol{\omega}_{B} \times \mathbf{J}\boldsymbol{\omega}_{B})   
\end{align*}
where $\mathbf{D} = \text{diag}(d_x, d_y, d_z)$ is a constant diagonal matrix that defines the rotor-drag coefficients
and $\mathbf{R}$ is the rotation matrix. 
% where $\mathbf{p}_{W}$ is the position, $\mathbf{v}_{W}$ is the linear velocity of the quadrotor in the world frame~${W}$,
% and $\mathbf{D} = \text{diag}(d_x, d_y, d_z)$ is a constant diagonal matrix that defines the rotor-drag coefficients, which is a linear effect in the quadrotor's velocity. 
% We use a unit quaternion $\mathbf{q}_{W}$ to represent the orientation of the quadrotor and 
% use $\boldsymbol{\omega}_{W}$ to denote the body rates in the body frame~${B}$.
Here, $\mathbf{g}=[0, 0, -g_z]^{T}$ with $g_z=\SI{9.81}{\meter\per\second\squared}$ is the gravity vector,
and $\mathbf{\Lambda} (\boldsymbol{\omega}_{B})$ is a skew-symmetric matrix.
Moreover, $\mathbf{c}=[0, 0, c]$ is the mass-normalized thrust vector. 
The conversion of single rotor thrusts $[f_1, f_2, f_3, f_4]$ to the mass-normalized thrust $c$ 
and the body torques $\boldsymbol{\eta}$ is formulated as
\begin{align}
    \boldsymbol{\eta} &= \begin{bmatrix}
    \frac{l}{\sqrt{2}}(f_1 - f_2 - f_3 + f_4)  \\ 
    \frac{l}{\sqrt{2}}(-f_1 - f_2 + f_3 + f_4) \\
    \kappa f_1 - \kappa f_2 + \kappa f_3 - \kappa f_4 \end{bmatrix} \\
   c &= (f_1 + f_2 + f_3 + f_4) / m
\end{align}
where $m$ is the quadrotor's mass and $l$ is the arm length.
We model the dynamics of a single-rotor thrust as first-order systems
$\dot{f} =(f_\text{des} - f)/ \alpha$ where $\alpha$ is the time-delay constant.
We use a 4th-order Runge-Kutta method for integrating the dynamic equations.
}

\subsection*{Hardware Design}
Table~\ref{tab: physical_drone} provides an overview of the hardware component configurations. We build our drone using off-the-shelf components that are easily available. Two types of physical drones have been developed for real-world deployment: the 4s drone and the 6s drone. These names derive from the number of battery cells they use (4 and 6 cells, respectively). The number of battery cells directly affects the maximum voltage applied to the motors and, consequently, the maximum force generated. The 4s drone can generate a maximum force of~\SI{34}{\newton}, whereas the 6s drone can produce up to~\SI{63}{\newton}. Compared to the 4s drone, the design of the 6s drone is more agile and compact, with reduced inertia and mass. These improvements result in a significant increase in the maximum thrust-to-weight ratio, from 4.62 to 12.45. To measure the maximum generated force, we used a load cell with a constant voltage supply. During real-world deployment, the actual voltage supply via an onboard battery usually fluctuates, resulting in lower total thrust.

Our quadrotor's frame consists of two types of carbon fiber, making the vehicle both durable and lightweight. The structural parts, excluding the frame, are custom-designed plastic components (made of PLA and TPU material) created using a 3D printer. PLA is used for most parts because of its stiffness, while TPU is used for impact protection and predetermined breaking points. To drive the quadrotor, we use fast-spinning brushless DC motors in conjunction with two types of 5.1-inch three-bladed propellers. Lithium-polymer batteries are employed to meet the high power demands of the motors. The motors are powered by an electronic speed controller that comes in a compact form and supports the DShot protocol for motor speed feedback. We use BetaFlight, an open-source software, as our low-level flight controller, as it offers real-time, low-latency control.

\subsection*{Related Work}

Given perfect state estimation, the conventional paradigm for autonomous racing is to decompose the solution into two stages: planning and control. 
For the planning stage, existing approaches in the context of quadrotors can be mostly categorized as polynomial approaches and optimization methods.
Polynomial trajectories~\cite{Mellinger11icra, Mellinger12ijrr, Richter2013ISRR} are efficient to generate and can leverage the differential flatness property of quadcopters.
Polynomial trajectories are limited to be smooth and are thus not always able to represent optimal control sequences, which may feature sharp mode switches, akin to bang-bang control \cite{Foehn2021science}.

Optimization-based trajectory planning allows for independently selecting the optimal sequence of states and control inputs at every time step, considering time minimization while complying with quadrotor dynamics and input constraints~\cite{Hehn12ar, Loock13ecc, Foehn2021science, Spedicato18tcst}.
Foehn et al.~\cite{Foehn2021science} introduced a complementary progress constraint (CPC) approach, which considers true actuator saturation, uses single rotor thrusts as control inputs, and exploits quaternions to allow full, singularity-free representation of the orientation space with consistent linearization characteristics.
While this method yields the optimal trajectory for a given quadrotor model, it is computationally expensive and is not tractable in real-time.

Previous studies\cite{Foehn2021science, Romero2021arxiv, Foehn20rss, de2022sensing, Wagter2021TheAI} have showcased remarkable advancements in autonomous drone racing using model-based control methods. 
Notably, Foehn et al.~\cite{Foehn2021science} demonstrated that it is possible to surpass two professional human pilots by proposing a time-optimal trajectory planning method, and then tracking it with a standard model predictive controller. 
However, i) the inherent nature of time-optimal trajectories and ii) the separation of the high-level task in planning and control hinder the capabilities of model-based control.
%present fundamental challenges to model-based control. 
%
The time-optimal trajectory given a dynamic system consists of control commands that lie mostly at the limit of actuation, leaving no extra control authority for the controller to counteract disturbances or model mismatches.
As a result, in order to track a time-optimal trajectory, Foehn et al.~\cite{Foehn2021science} needed to lower the effective thrust limit to 70\% of the maximum available thrust when deploying their system in the real world.
For a fair comparison against professional human pilots, the quadrotor platform used for human flights was reduced to the same thrust-to-weight ratio as the autonomous platform~\cite{Foehn2021science}.

Learning-based approaches to autonomous racing replace the planning and control stack with a neural network~\cite{Loquercio19TRO,kaufmann2022benchmark}.
Purely data-driven control strategies, such as model-free reinforcement learning, aim to circumvent the limitations of model-based controller design by learning effective controllers directly from experience.
For example, control of a physical quadrotor using reinforcement learning was demonstrated by Hwangbo et al.~\cite{hwangbo2017control}, who used a neural network policy to track waypoints and recover from challenging initialization.  
Koch et al.~\cite{koch2019reinforcement} applied model-free RL to low-level attitude control and showed that a learned low-level controller trained with PPO outperformed a fully tuned PID controller on almost every metric.
Song et al.~\cite{song2021autonomous} used deep RL to generate near-time-optimal trajectories for autonomous drone racing and tracked the trajectories by an MPC controller. 
Lambert et al.~\cite{lambert2019low} used model-based RL to train a hovering controller. 
\newpage

\subsection*{Supplementary Figures}
\input{Images/objectives_tikz.tex}

\begin{figure}[htp]
    \includegraphics[width=1.0\linewidth]{Images/training_curve.pdf}
    \caption{ \textbf{Learning curves for gate progress maximization, averaged across 10 runs with different seeds.}  We compute the mean (solid line) and standard deviation (shadow region). Each policy is trained for a total of 25 million simulation timesteps. The total training time for every single policy takes around 10 minutes. We use a desktop computer equipped with an Intel i9-9900K CPU and an Nvidia Titan RTX graphics card.}
    \label{fig: training_curve}
\end{figure}

% \begin{figure}[!htp]
% \begin{tikzpicture}
% \node at (0,0) (main) [text width = 1.0\linewidth] {
%     \fontsize{9pt}{12pt}\selectfont
%     \begin{center}
% 

%     \end{center}
%     };
%     \end{tikzpicture}
%     \caption{Overview of the racing drone configurations for real-world experiments.}
%     \label{tab:physical_drone}
% \end{figure}

\newpage
\subsection*{Supplementary Tables}

\begin{table}[!htb] 
   \centering 
    \fontsize{9pt}{12pt}\selectfont
    \begin{tabular}{c}
        \begin{tabular}{c|c}
            \begin{subfigure}[t]{0.4\textwidth}
                 \captionsetup{labelformat=empty}
                 \caption{\textbf{4s Drone}}
                 \includegraphics[width=1\linewidth]{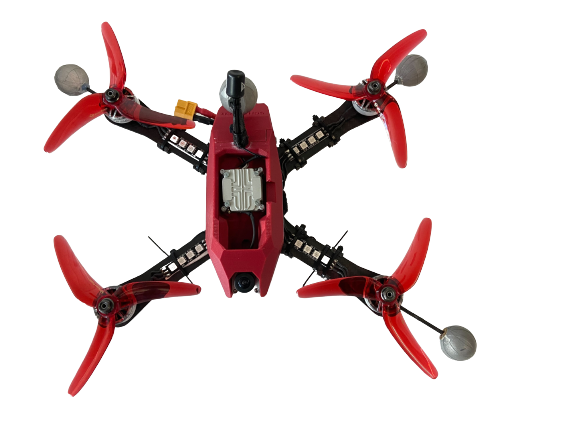}
            \end{subfigure} &
            \begin{subfigure}[t]{0.4\textwidth}
                 \captionsetup{labelformat=empty}
                 \caption{\textbf{6s Drone}}
                 \includegraphics[width=1\linewidth]{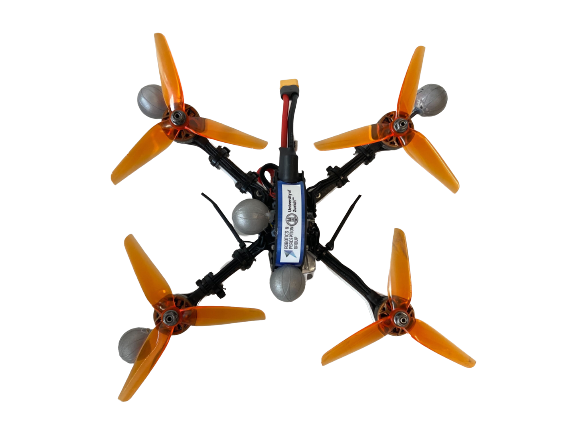}
            \end{subfigure} 
        \end{tabular}     
    \end{tabular}
    \begin{tabular}{ l | c | c}
        \toprule
          \textbf{Parameters}  & \textbf{4s Drone}  & \textbf{6s Drone} \\ \cline{1-3}
          Thrust-to-weight Ratio   & 4.62 & 12.45 \\
          Mass [\SI{}{\kilogram}]   &  0.75 & 0.52 \\
          Maximum Thrust [\SI{}{\newton}]  & 34.00  & 63.76 \\
          Arm Length [\SI{}{\meter}]  & 0.15 & 0.11\\
          Inertia  [\SI{}{\gram\square\meter}]  & [2.50, 2.51, 4.32] & [1.37, 1.34, 2.45]\\
          Motor Time Constant [\SI{}{\second}]  & 0.033  & 0.020 \\ \toprule
        \textbf{Components}  & \textbf{4s Drone}  & \textbf{6s Drone} \\ \hline
          Frame &Chameleon 6 inch &BMSRacing JS-1  \\
          Motor & Xrotor 2306 & BMS Raptor V2  \\
          Propeller & Azure Power SFP 5148 5 & HQ Prop R42 \\
          Flight Controller & BrainFPV radix & Foxeer Mini F722 \\
          Battery & Tattu 4 cells 1800 mAh & Tattu 6 cells 1300 mAh  \\
          Electronic Speed Controller (ESC) &  Hobbywing XRotor & Foxeer Reaper Mini 128K \\ 
        \bottomrule
    \end{tabular}
   % \vspace{0.5em} 
   \caption{\textbf{Overview of the racing drone configurations for real-world experiments.} The 4s Drone is used for the baseline comparison between our RL policy and optimal control methods. The 6s Drone is used for pushing the limit of our RL controller in the physical world and for the competition against human pilots. } 
   \label{tab: physical_drone}
\end{table} 

\begin{table}[!htb] 
   \centering 
    \fontsize{9pt}{12pt}\selectfont
    \begin{tabular}{ l | c }
        \toprule
          \textbf{Parameter}  & \textbf{Value}  \\
          \hline 
          learning rate   &  0.0003 \\
          discount factor & 0.99\\
          GAE-$\lambda$ & 0.95 \\
          learning epoch & 10 \\
          policy network & MLP [512, 512] \\
          value network & MLP [512, 512]  \\
          clip range & 0.2 \\
          entropy coefficient & 0.005 \\
          batch size & 25000\\
        \bottomrule
    \end{tabular}
   % \vspace{0.5em} 
   \caption{\textbf{PPO hyperparameters.} We train the policy using Proximal Policy Optimization (PPO). We simulate 100 environments in parallel to collect rollouts. We use the running mean and standard deviation to normalize the observation. MLP represents a multilayer perceptron network, and GAE represents generalized advantage estimate} 
   \label{tab: hyperparameters}
\end{table} 

\begin{table}[!htb] 
   \centering 
    \fontsize{9pt}{12pt}\selectfont
    \begin{tabular}{c | c}
        \begin{subfigure}[t]{0.45\textwidth}
             \captionsetup{labelformat=empty}
             \caption{\textbf{Split-S Track}}
             \includegraphics[width=1\linewidth]{Images/splits_drone.png}
        \end{subfigure} &
        \begin{subfigure}[t]{0.45\textwidth}
             \captionsetup{labelformat=empty}
             \caption{\textbf{Marv Track}}
             \includegraphics[width=1\linewidth]{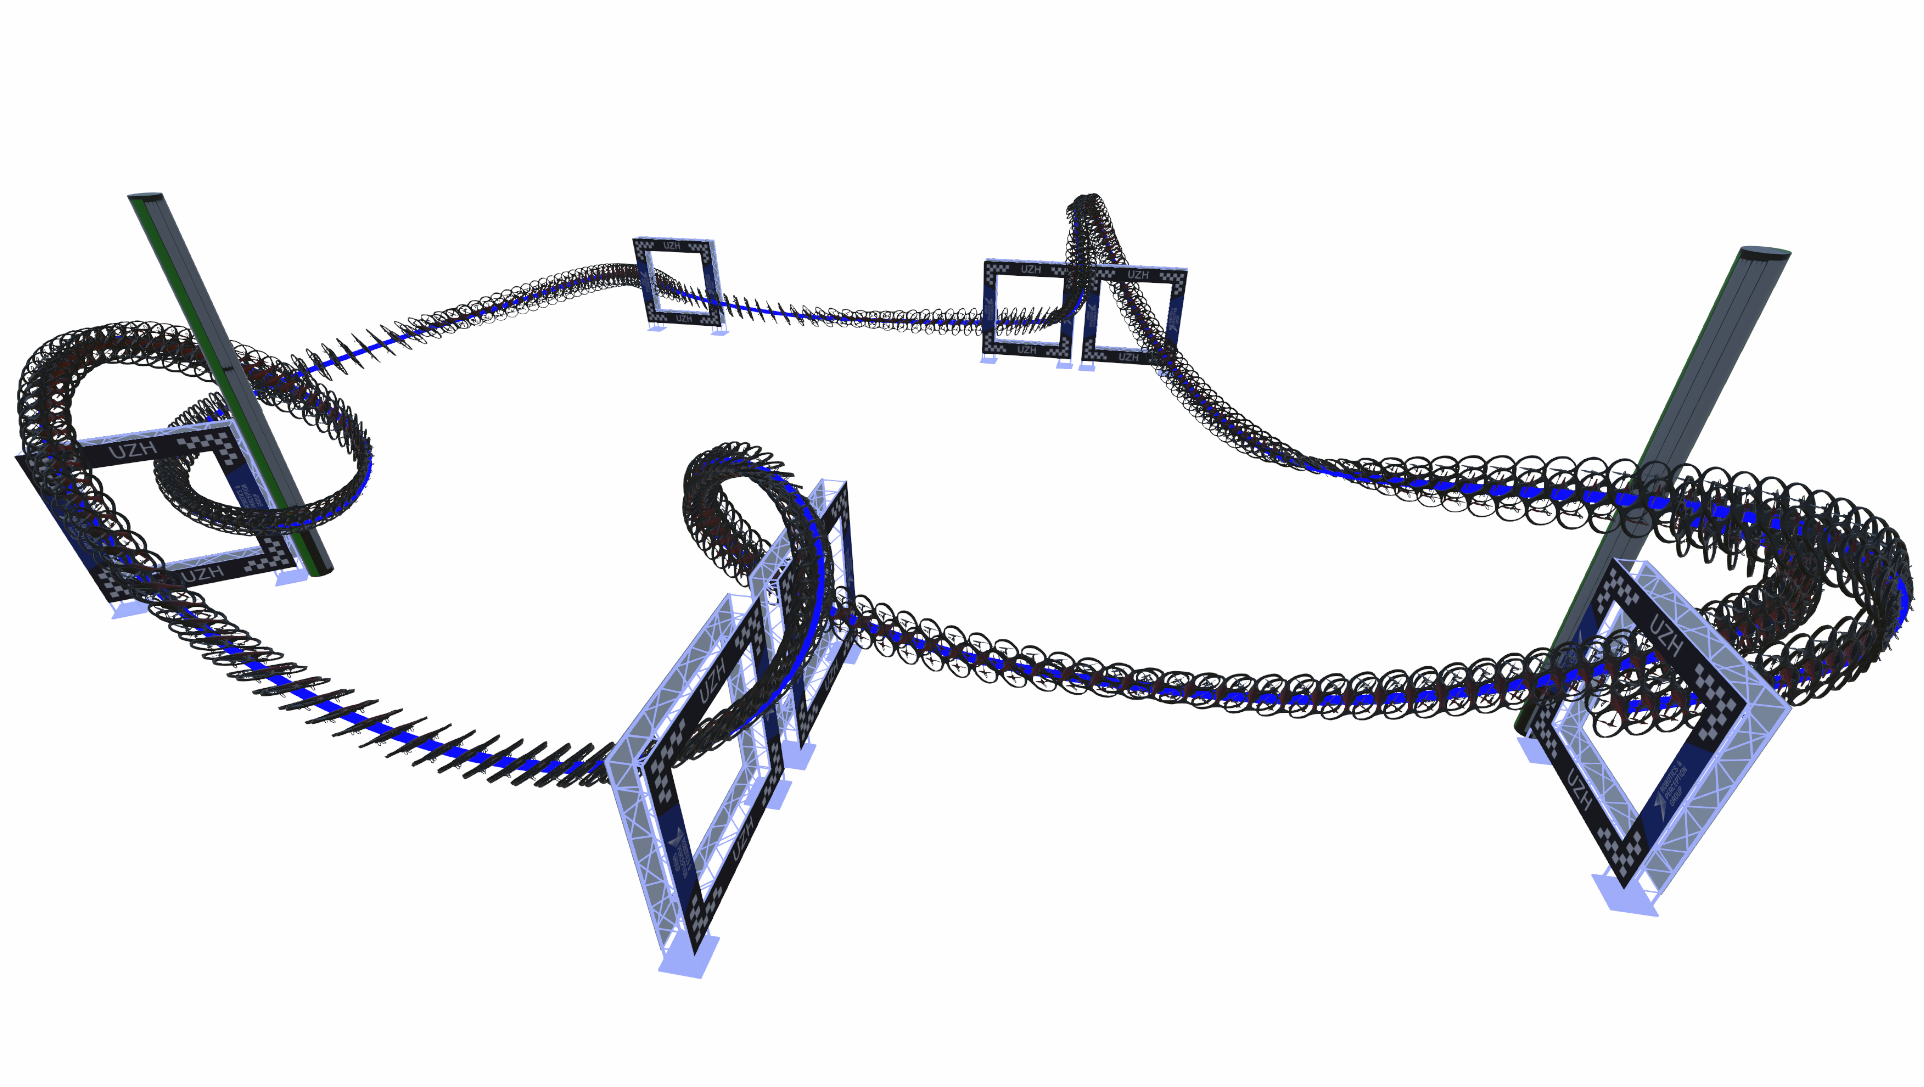}
        \end{subfigure} 
    \end{tabular}
    \begin{tabular}{ l | c | c | c  }
        \toprule
          \textbf{Split-S Track}  & \textbf{Gate Center} ($x, y, z$) & \textbf{Orientation} $(q_w, q_x, q_y, q_z)$ & \textbf{Depth $\times$ Width $\times$ Height} (\SI{}{\meter})  \\
          \hline
          Gate 1 & [-0.70, -0.89, 3.53] & [0.96, 0.0, 0.0, -0.27] & [0.2 $\times$ 1.5 $\times$ 1.5]\\
          Gate 2 & [9.17, 6.25, 1.12] & [1.0, 0.0, 0.0, 0.0] & [0.2 $\times$ 1.5 $\times$ 1.5]\\
          Gate 3 & [8.90, -3.81, 1.12] & [-0.44, 0.0, 0.0, 0.90] & [0.2 $\times$ 1.5 $\times$ 1.5]\\
          Gate 4 & [-4.40, -5.77, 3.20] & [0.0, 0.0, 0.0, 1.0] & [0.2 $\times$ 1.5 $\times$ 1.5]\\
          Gate 5 & [-4.40, -5.79, 1.12] & [1.0, 0.0, 0.0, 0.0] & [0.2 $\times$ 1.5 $\times$ 1.5]\\
          Gate 6 & [4.48, -0.46, 1.12] & [0.67, 0.0, 0.0, 0.74] & [0.2 $\times$ 1.5 $\times$ 1.5]\\
          Gate 7 & [-1.94, 6.82, 1.12] & [-0.26, 0.0, 0.0, 0.97] & [0.2 $\times$ 1.5 $\times$ 1.5]\\
        \midrule
         \textbf{Marv Track}  & \textbf{Gate Center} ($x, y, z$) & \textbf{Orientation} $(q_w, q_x, q_y, q_z)$ & \textbf{Depth $\times$ Width $\times$ Height} (\SI{}{\meter})  \\
          \hline
          Gate 1 & [7.70, 11.46, 1.12] & [0.72, 0.0, 0.0, -0.70] & [0.2 $\times$ 1.5 $\times$ 1.5]\\
          Gate 2 & [7.57, 3.97, 1.12] & [0.71, 0.0, 0.0, -0.70] & [0.2 $\times$ 1.5 $\times$ 1.5]\\
          Gate 3 & [9.88, 3.97, 1.12] & [0.72, 0.0, 0.0, -0.70] & [0.2 $\times$ 1.5 $\times$ 1.5]\\
          Gate 4 & [7.15, -4.78, 1.12] & [-0.33, 0.0, 0.0, 0.94] & [0.2 $\times$ 1.5 $\times$ 1.5]\\
          Gate 5 & [-5.51, -4.32, 1.12] & [1.0, 0.0, 0.0, 0.0] & [0.2 $\times$ 1.5 $\times$ 1.5]\\
          Gate 6 & [-4.60, 4.53, 1.12] & [1.0, 0.0, 0.0, 0.0] & [0.2 $\times$ 1.5 $\times$ 1.5]\\
          Gate 7 & [-4.60, 6.79, 1.12] & [1.0, 0.0, 0.0, 0.0] & [0.2 $\times$ 1.5 $\times$ 1.5]\\
        \bottomrule
    \end{tabular}
   % \vspace{0.5em} 
   \caption{\textbf{Race track configurations.} Both tracks have in total of 7 gates, but the gates are arranged in different configurations. We consider all gates to have a rectangular shape with the same dimension. The Split-S track contains two vertically stacked gates, which require a so-called Split-S manoeuvre. The Marv track features more challenging maneuvers commonly used in FPV drone racing, including one Split-S manoeuvre, two power-loop manoeuvres, one ladder manoeuvre, and one hairpin manoeuvre. } 
   \label{tab: race_track_config}
\end{table} 

\clearpage

\final{
\subsection*{Supplementary Movies}
\noindent Movie S1. An overview of the methodology and results. \\
\noindent Movie S2. An animation of policy training in simulation. \\
\noindent Movie S3. Deployment of the reinforcement learning policy in the SplitS track. \\
\noindent Movie S4. Deployment of the reinforcement learning policy in the Marv track.
}
